# Supplementary material for: Learning Shape Templates with Structured Implicit Functions
Source: arXiv:1904.06447 source file (2019-04-12)
Supplement: Supplementary file 1 [file qual_results.tex]

\section{Additional Template Fitting Results}

We provide qualitative template fitting results for all 13 classes in Figures~\ref{fig:airplane_qual}-\ref{fig:watercraft_qual}. We show the first few models per class based on their alphabetical order. For each example, we show both the single class result and the multiclass result. The multiclass result is from the same network across all 13 classes. For single class results, there is one network trained per class. The per class networks are trained with identical hyperparameters; the only difference is the input data. In the majority of cases, we see improvements in detail when training single class as compared to multiclass.

These results provide several insights into the performance and failure cases of the model. First, there is a large gap in reconstruction performance between the train and test set. There are a variety of explanations for this, although one likely issue is insufficient training data. The train splits have only a few hundred to a few thousand (or 30,000, for multi-class) examples in them, depending on the class or set of classes being trained on.  Dataset augmentation or a larger dataset might help improve generalization.

Another weakness is that some shapes that are very unusual, such as the second training set bench in Figure~\ref{fig:bench_qual}, can be difficult to fit because the template does not easily accomodate them. Finally, it is important to note that training relies on reasonably aligned data, so for examples where the data is out of alignment, performance can be poor. One example can be seen in the video, where a sofa is backwards- this causes the shape element correspondence to be weaker and for interpolation to produce an abrupt result.

\begin{figure*}
    \centering
        \begin{tabular}{ccccc}
        & \multicolumn{2}{c}{Multiclass Model: Train} & \multicolumn{2}{c}{Singleclass Model: Train}\\
        \hline
        ~~~~~~~Input Mesh~~~~~~~~~& ~~~~~~~Template~~~~~~~~ & ~~~~~~~Isosurface~~~~~~~~ & ~~~~~~~~Template~~~~~~ & Isosurface\\
        \multicolumn{5}{c}{\adjincludegraphics[width=0.9\textwidth, trim={0 {0.0\height} 0 0}, clip]{image/reconstruction/reconstruction_airplane_train.png}}\\
        & \multicolumn{2}{c}{Multiclass Model: Test} & \multicolumn{2}{c}{Singleclass Model: Test}\\
        \hline
        ~~~~~~~Input Mesh~~~~~~~~~& ~~~~~~~Template~~~~~~~~ & ~~~~~~~Isosurface~~~~~~~~ & ~~~~~~~~Template~~~~~~ & Isosurface\\
         \multicolumn{5}{c}{\adjincludegraphics[width=0.9\textwidth, trim={0 {0.0\height} 0 0}, clip]{image/reconstruction/reconstruction_airplane_test.png}}\\    
        
    \end{tabular}
    \caption{Template fitting results for ShapeNet class ``\textbf{airplane}'' with 100 shape elements. The first models alphabetically are shown.}
    \vspace{1cm}
    \label{fig:airplane_qual}
\end{figure*}

\begin{figure*}
    \centering
        \begin{tabular}{ccccc}
        & \multicolumn{2}{c}{Multiclass Model: Train} & \multicolumn{2}{c}{Singleclass Model: Train}\\
        \hline
        ~~~~~~~Input Mesh~~~~~~~~~& ~~~~~~~Template~~~~~~~~ & ~~~~~~~Isosurface~~~~~~~~ & ~~~~~~~~Template~~~~~~ & Isosurface\\
        \multicolumn{5}{c}{\adjincludegraphics[width=0.9\textwidth, trim={0 {0.0\height} 0 0}, clip]{image/reconstruction/reconstruction_bench_train.png}}\\
        & \multicolumn{2}{c}{Multiclass Model: Test} & \multicolumn{2}{c}{Singleclass Model: Test}\\
        \hline
        ~~~~~~~Input Mesh~~~~~~~~~& ~~~~~~~Template~~~~~~~~ & ~~~~~~~Isosurface~~~~~~~~ & ~~~~~~~~Template~~~~~~ & Isosurface\\
         \multicolumn{5}{c}{\adjincludegraphics[width=0.9\textwidth, trim={0 {0.0\height} 0 0}, clip]{image/reconstruction/reconstruction_bench_test.png}}\\    
        
    \end{tabular}
    \caption{Template fitting results for ShapeNet class ``\textbf{bench}'' with 100 shape elements. The first models alphabetically are shown.}
    \vspace{1cm}
    \label{fig:bench_qual}
\end{figure*}

\begin{figure*}
    \centering
        \begin{tabular}{ccccc}
        & \multicolumn{2}{c}{Multiclass Model: Train} & \multicolumn{2}{c}{Singleclass Model: Train}\\
        \hline
        ~~~~~~~Input Mesh~~~~~~~~~& ~~~~~~~Template~~~~~~~~ & ~~~~~~~Isosurface~~~~~~~~ & ~~~~~~~~Template~~~~~~ & Isosurface\\
        \multicolumn{5}{c}{\adjincludegraphics[width=0.9\textwidth, trim={0 {0.0\height} 0 0}, clip]{image/reconstruction/reconstruction_cabinet_train.png}}\\
        & \multicolumn{2}{c}{Multiclass Model: Test} & \multicolumn{2}{c}{Singleclass Model: Test}\\
        \hline
        ~~~~~~~Input Mesh~~~~~~~~~& ~~~~~~~Template~~~~~~~~ & ~~~~~~~Isosurface~~~~~~~~ & ~~~~~~~~Template~~~~~~ & Isosurface\\
         \multicolumn{5}{c}{\adjincludegraphics[width=0.9\textwidth, trim={0 {0.0\height} 0 0}, clip]{image/reconstruction/reconstruction_cabinet_test.png}}\\    
        
    \end{tabular}
    \caption{Template fitting results for ShapeNet class ``\textbf{cabinet}'' with 100 shape elements. The first models alphabetically are shown.}
    \vspace{1cm}
    \label{fig:cabinet_qual}
\end{figure*}

\begin{figure*}
    \centering
        \begin{tabular}{ccccc}
        & \multicolumn{2}{c}{Multiclass Model: Train} & \multicolumn{2}{c}{Singleclass Model: Train}\\
        \hline
        ~~~~~~~Input Mesh~~~~~~~~~& ~~~~~~~Template~~~~~~~~ & ~~~~~~~Isosurface~~~~~~~~ & ~~~~~~~~Template~~~~~~ & Isosurface\\
        \multicolumn{5}{c}{\adjincludegraphics[width=0.9\textwidth, trim={0 {0.0\height} 0 0}, clip]{image/reconstruction/reconstruction_car_train.png}}\\
        & \multicolumn{2}{c}{Multiclass Model: Test} & \multicolumn{2}{c}{Singleclass Model: Test}\\
        \hline
        ~~~~~~~Input Mesh~~~~~~~~~& ~~~~~~~Template~~~~~~~~ & ~~~~~~~Isosurface~~~~~~~~ & ~~~~~~~~Template~~~~~~ & Isosurface\\
         \multicolumn{5}{c}{\adjincludegraphics[width=0.9\textwidth, trim={0 {0.0\height} 0 0}, clip]{image/reconstruction/reconstruction_car_test.png}}\\    
        
    \end{tabular}
    \caption{Template fitting results for ShapeNet class ``\textbf{car}'' with 100 shape elements. The first models alphabetically are shown.}
    \vspace{1cm}
    \label{fig:car_qual}
\end{figure*}

\begin{figure*}
    \centering
        \begin{tabular}{ccccc}
        & \multicolumn{2}{c}{Multiclass Model: Train} & \multicolumn{2}{c}{Singleclass Model: Train}\\
        \hline
        ~~~~~~~Input Mesh~~~~~~~~~& ~~~~~~~Template~~~~~~~~ & ~~~~~~~Isosurface~~~~~~~~ & ~~~~~~~~Template~~~~~~ & Isosurface\\
        \multicolumn{5}{c}{\adjincludegraphics[width=0.9\textwidth, trim={0 {0.0\height} 0 0}, clip]{image/reconstruction/reconstruction_chair_train.png}}\\
        & \multicolumn{2}{c}{Multiclass Model: Test} & \multicolumn{2}{c}{Singleclass Model: Test}\\
        \hline
        ~~~~~~~Input Mesh~~~~~~~~~& ~~~~~~~Template~~~~~~~~ & ~~~~~~~Isosurface~~~~~~~~ & ~~~~~~~~Template~~~~~~ & Isosurface\\
         \multicolumn{5}{c}{\adjincludegraphics[width=0.9\textwidth, trim={0 {0.0\height} 0 0}, clip]{image/reconstruction/reconstruction_chair_test.png}}\\    
        
    \end{tabular}
    \caption{Template fitting results for ShapeNet class ``\textbf{chair}'' with 100 shape elements. The first models alphabetically are shown.}
    \vspace{1cm}
    \label{fig:chair_qual}
\end{figure*}

\begin{figure*}
    \centering
        \begin{tabular}{ccccc}
        & \multicolumn{2}{c}{Multiclass Model: Train} & \multicolumn{2}{c}{Singleclass Model: Train}\\
        \hline
        ~~~~~~~Input Mesh~~~~~~~~~& ~~~~~~~Template~~~~~~~~ & ~~~~~~~Isosurface~~~~~~~~ & ~~~~~~~~Template~~~~~~ & Isosurface\\
        \multicolumn{5}{c}{\adjincludegraphics[width=0.9\textwidth, trim={0 {0.0\height} 0 0}, clip]{image/reconstruction/reconstruction_display_train.png}}\\
        & \multicolumn{2}{c}{Multiclass Model: Test} & \multicolumn{2}{c}{Singleclass Model: Test}\\
        \hline
        ~~~~~~~Input Mesh~~~~~~~~~& ~~~~~~~Template~~~~~~~~ & ~~~~~~~Isosurface~~~~~~~~ & ~~~~~~~~Template~~~~~~ & Isosurface\\
         \multicolumn{5}{c}{\adjincludegraphics[width=0.9\textwidth, trim={0 {0.0\height} 0 0}, clip]{image/reconstruction/reconstruction_display_test.png}}\\    
        
    \end{tabular}
    \caption{Template fitting results for ShapeNet class ``\textbf{display}'' with 100 shape elements. The first models alphabetically are shown.}
    \vspace{1cm}
    \label{fig:display_qual}
\end{figure*}

\begin{figure*}
    \centering
        \begin{tabular}{ccccc}
        & \multicolumn{2}{c}{Multiclass Model: Train} & \multicolumn{2}{c}{Singleclass Model: Train}\\
        \hline
        ~~~~~~~Input Mesh~~~~~~~~~& ~~~~~~~Template~~~~~~~~ & ~~~~~~~Isosurface~~~~~~~~ & ~~~~~~~~Template~~~~~~ & Isosurface\\
        \multicolumn{5}{c}{\adjincludegraphics[width=0.9\textwidth, trim={0 {0.0\height} 0 0}, clip]{image/reconstruction/reconstruction_lamp_train.png}}\\
        & \multicolumn{2}{c}{Multiclass Model: Test} & \multicolumn{2}{c}{Singleclass Model: Test}\\
        \hline
        ~~~~~~~Input Mesh~~~~~~~~~& ~~~~~~~Template~~~~~~~~ & ~~~~~~~Isosurface~~~~~~~~ & ~~~~~~~~Template~~~~~~ & Isosurface\\
         \multicolumn{5}{c}{\adjincludegraphics[width=0.9\textwidth, trim={0 {0.0\height} 0 0}, clip]{image/reconstruction/reconstruction_lamp_test.png}}\\    
        
    \end{tabular}
    \caption{Template fitting results for ShapeNet class ``\textbf{lamp}'' with 100 shape elements. The first models alphabetically are shown.}
    \vspace{1cm}
    \label{fig:lamp_qual}
\end{figure*}

\begin{figure*}
    \centering
        \begin{tabular}{ccccc}
        & \multicolumn{2}{c}{Multiclass Model: Train} & \multicolumn{2}{c}{Singleclass Model: Train}\\
        \hline
        ~~~~~~~Input Mesh~~~~~~~~~& ~~~~~~~Template~~~~~~~~ & ~~~~~~~Isosurface~~~~~~~~ & ~~~~~~~~Template~~~~~~ & Isosurface\\
        \multicolumn{5}{c}{\adjincludegraphics[width=0.9\textwidth, trim={0 {0.0\height} 0 0}, clip]{image/reconstruction/reconstruction_rifle_train.png}}\\
        & \multicolumn{2}{c}{Multiclass Model: Test} & \multicolumn{2}{c}{Singleclass Model: Test}\\
        \hline
        ~~~~~~~Input Mesh~~~~~~~~~& ~~~~~~~Template~~~~~~~~ & ~~~~~~~Isosurface~~~~~~~~ & ~~~~~~~~Template~~~~~~ & Isosurface\\
         \multicolumn{5}{c}{\adjincludegraphics[width=0.9\textwidth, trim={0 {0.0\height} 0 0}, clip]{image/reconstruction/reconstruction_rifle_test.png}}\\    
        
    \end{tabular}
    \caption{Template fitting results for ShapeNet class ``\textbf{rifle}'' with 100 shape elements. The first models alphabetically are shown.}
    \vspace{1cm}
    \label{fig:rifle_qual}
\end{figure*}

\begin{figure*}
    \centering
        \begin{tabular}{ccccc}
        & \multicolumn{2}{c}{Multiclass Model: Train} & \multicolumn{2}{c}{Singleclass Model: Train}\\
        \hline
        ~~~~~~~Input Mesh~~~~~~~~~& ~~~~~~~Template~~~~~~~~ & ~~~~~~~Isosurface~~~~~~~~ & ~~~~~~~~Template~~~~~~ & Isosurface\\
        \multicolumn{5}{c}{\adjincludegraphics[width=0.9\textwidth, trim={0 {0.0\height} 0 0}, clip]{image/reconstruction/reconstruction_sofa_train.png}}\\
        & \multicolumn{2}{c}{Multiclass Model: Test} & \multicolumn{2}{c}{Singleclass Model: Test}\\
        \hline
        ~~~~~~~Input Mesh~~~~~~~~~& ~~~~~~~Template~~~~~~~~ & ~~~~~~~Isosurface~~~~~~~~ & ~~~~~~~~Template~~~~~~ & Isosurface\\
         \multicolumn{5}{c}{\adjincludegraphics[width=0.9\textwidth, trim={0 {0.0\height} 0 0}, clip]{image/reconstruction/reconstruction_sofa_test.png}}\\    
        
    \end{tabular}
    \caption{Template fitting results for ShapeNet class ``\textbf{sofa}'' with 100 shape elements. The first models alphabetically are shown.}
    \vspace{1cm}
    \label{fig:sofa_qual}
\end{figure*}

\begin{figure*}
    \centering
        \begin{tabular}{ccccc}
        & \multicolumn{2}{c}{Multiclass Model: Train} & \multicolumn{2}{c}{Singleclass Model: Train}\\
        \hline
        ~~~~~~~Input Mesh~~~~~~~~~& ~~~~~~~Template~~~~~~~~ & ~~~~~~~Isosurface~~~~~~~~ & ~~~~~~~~Template~~~~~~ & Isosurface\\
        \multicolumn{5}{c}{\adjincludegraphics[width=0.9\textwidth, trim={0 {0.0\height} 0 0}, clip]{image/reconstruction/reconstruction_speaker_train.png}}\\
        & \multicolumn{2}{c}{Multiclass Model: Test} & \multicolumn{2}{c}{Singleclass Model: Test}\\
        \hline
        ~~~~~~~Input Mesh~~~~~~~~~& ~~~~~~~Template~~~~~~~~ & ~~~~~~~Isosurface~~~~~~~~ & ~~~~~~~~Template~~~~~~ & Isosurface\\
         \multicolumn{5}{c}{\adjincludegraphics[width=0.9\textwidth, trim={0 {0.0\height} 0 0}, clip]{image/reconstruction/reconstruction_speaker_test.png}}\\    
        
    \end{tabular}
    \caption{Template fitting results for ShapeNet class ``\textbf{speaker}'' with 100 shape elements. The first models alphabetically are shown.}
    \vspace{1cm}
    \label{fig:speaker_qual}
\end{figure*}

\begin{figure*}
    \centering
        \begin{tabular}{ccccc}
        & \multicolumn{2}{c}{Multiclass Model: Train} & \multicolumn{2}{c}{Singleclass Model: Train}\\
        \hline
        ~~~~~~~Input Mesh~~~~~~~~~& ~~~~~~~Template~~~~~~~~ & ~~~~~~~Isosurface~~~~~~~~ & ~~~~~~~~Template~~~~~~ & Isosurface\\
        \multicolumn{5}{c}{\adjincludegraphics[width=0.9\textwidth, trim={0 {0.0\height} 0 0}, clip]{image/reconstruction/reconstruction_table_train.png}}\\
        & \multicolumn{2}{c}{Multiclass Model: Test} & \multicolumn{2}{c}{Singleclass Model: Test}\\
        \hline
        ~~~~~~~Input Mesh~~~~~~~~~& ~~~~~~~Template~~~~~~~~ & ~~~~~~~Isosurface~~~~~~~~ & ~~~~~~~~Template~~~~~~ & Isosurface\\
         \multicolumn{5}{c}{\adjincludegraphics[width=0.9\textwidth, trim={0 {0.0\height} 0 0}, clip]{image/reconstruction/reconstruction_table_test.png}}\\    
        
    \end{tabular}
    \caption{Template fitting results for ShapeNet class ``\textbf{table}'' with 100 shape elements. The first models alphabetically are shown.}
    \vspace{1cm}
    \label{fig:table_qual}
\end{figure*}

\begin{figure*}
    \centering
        \begin{tabular}{ccccc}
        & \multicolumn{2}{c}{Multiclass Model: Train} & \multicolumn{2}{c}{Singleclass Model: Train}\\
        \hline
        ~~~~~~~Input Mesh~~~~~~~~~& ~~~~~~~Template~~~~~~~~ & ~~~~~~~Isosurface~~~~~~~~ & ~~~~~~~~Template~~~~~~ & Isosurface\\
        \multicolumn{5}{c}{\adjincludegraphics[width=0.9\textwidth, trim={0 {0.0\height} 0 0}, clip]{image/reconstruction/reconstruction_telephone_train.png}}\\
        & \multicolumn{2}{c}{Multiclass Model: Test} & \multicolumn{2}{c}{Singleclass Model: Test}\\
        \hline
        ~~~~~~~Input Mesh~~~~~~~~~& ~~~~~~~Template~~~~~~~~ & ~~~~~~~Isosurface~~~~~~~~ & ~~~~~~~~Template~~~~~~ & Isosurface\\
         \multicolumn{5}{c}{\adjincludegraphics[width=0.9\textwidth, trim={0 {0.0\height} 0 0}, clip]{image/reconstruction/reconstruction_telephone_test.png}}\\    
        
    \end{tabular}
    \caption{Template fitting results for ShapeNet class ``\textbf{telephone}'' with 100 shape elements. The first models alphabetically are shown.}
    \vspace{1cm}
    \label{fig:telephone_qual}
\end{figure*}

\begin{figure*}
    \centering
        \begin{tabular}{ccccc}
        & \multicolumn{2}{c}{Multiclass Model: Train} & \multicolumn{2}{c}{Singleclass Model: Train}\\
        \hline
        ~~~~~~~Input Mesh~~~~~~~~~& ~~~~~~~Template~~~~~~~~ & ~~~~~~~Isosurface~~~~~~~~ & ~~~~~~~~Template~~~~~~ & Isosurface\\
        \multicolumn{5}{c}{\adjincludegraphics[width=0.9\textwidth, trim={0 {0.0\height} 0 0}, clip]{image/reconstruction/reconstruction_watercraft_train.png}}\\
        & \multicolumn{2}{c}{Multiclass Model: Test} & \multicolumn{2}{c}{Singleclass Model: Test}\\
        \hline
        ~~~~~~~Input Mesh~~~~~~~~~& ~~~~~~~Template~~~~~~~~ & ~~~~~~~Isosurface~~~~~~~~ & ~~~~~~~~Template~~~~~~ & Isosurface\\
         \multicolumn{5}{c}{\adjincludegraphics[width=0.9\textwidth, trim={0 {0.0\height} 0 0}, clip]{image/reconstruction/reconstruction_watercraft_test.png}}\\    
        
    \end{tabular}
    \caption{Template fitting results for ShapeNet class ``\textbf{watercraft}'' with 100 shape elements. The first models alphabetically are shown.}
    \vspace{1cm}
    \label{fig:watercraft_qual}
\end{figure*}
